# Supplementary material for: A Systematic Evaluation of Co-folding Model Representations for Small-Molecule Learning
Source: arXiv:2602.13249 source file (2026-05-22)
Supplement: Supplementary file 1 [file tab_time.tex]

\begin{table}[h]
\caption{\textbf{Inference time of Boltz2 trunk module for processing a molecule.} We consider three recycling steps. We consider a single NVIDIA B200 GPU.}
\label{tab:inference_time}
\centering
\setlength{\tabcolsep}{10pt}
\begin{tabular}{c c c c}
\toprule
\textbf{Batch size} &
\textbf{Inference time} &
\textbf{Throughput} &
\textbf{Peak GPU memory} \\
\midrule
1 & 1030.90 ms/mol (1030.90 ms) & 0.97 mol/s & 1,996 MB \\
1{,}000 & 16.74 ms/mol (16738.76 ms) & 59.74 mol/s & 88{,}590 MB \\
\bottomrule
\end{tabular}
\end{table}
